# Supplementary material for: Unexpected Anisotropic Mn-Sb Anti-site Distribution and Van der Waals Epitaxy of MnSb2Te4
Source: arXiv:2601.11353 source file (2026-01-16)
Supplement: Supplementary file 1 [file SupplementaryMaterialVersion2.pdf]

# **Supporting Information of: Unexpected Anisotropic Mn-Sb Anti-site Distribution and Van der Waals Epitaxy of MnSb<sub>2</sub>Te<sub>4</sub>**

by Gustavo Chavez Ponce de Leon ([g.ponce.de.leon@rug.nl](mailto:g.ponce.de.leon@rug.nl)), Ahmad Dibajeh ([a.j.f.dibajeh@rug.nl](mailto:a.j.f.dibajeh@rug.nl)), Gert ten Brink ([g.h.ten.brink@rug.nl](mailto:g.h.ten.brink@rug.nl)), Majid Ahmadi ([majid.ahmadi@rug.nl](mailto:majid.ahmadi@rug.nl)), Bart Jan Kooi ([b.j.kooi@rug.nl](mailto:b.j.kooi@rug.nl)), George Palasantzas ([g.palasantzas@rug.nl](mailto:g.palasantzas@rug.nl)).

## **Content**

S1: XRD of powder samples from different parts of the ingot

S2: Detailed structural analysis of STEM pictures

S3: RHEED data of additional thin film depositions

S4: EDS of solid ingot

S5: Additional atomically-resolved EDS maps (ingot and thin film)

S6: Additional magnetization plots

### S1: XRD of powder samples from different parts of the ingot

To confirm the uniformity of the synthesized ingot, powder samples were collected from different parts hereby named: top, middle, bottom. Their respective XRD spectrum are plotted in **Figure S1**. The position and intensity of all peaks are consistent with each other.

The morphology of the powder was “flake-like” (see **Figure 1b** of the main text); thus, the relative peak amplitude measured experimentally is expected to differ from the theoretical values, which assume an isotropic powder.

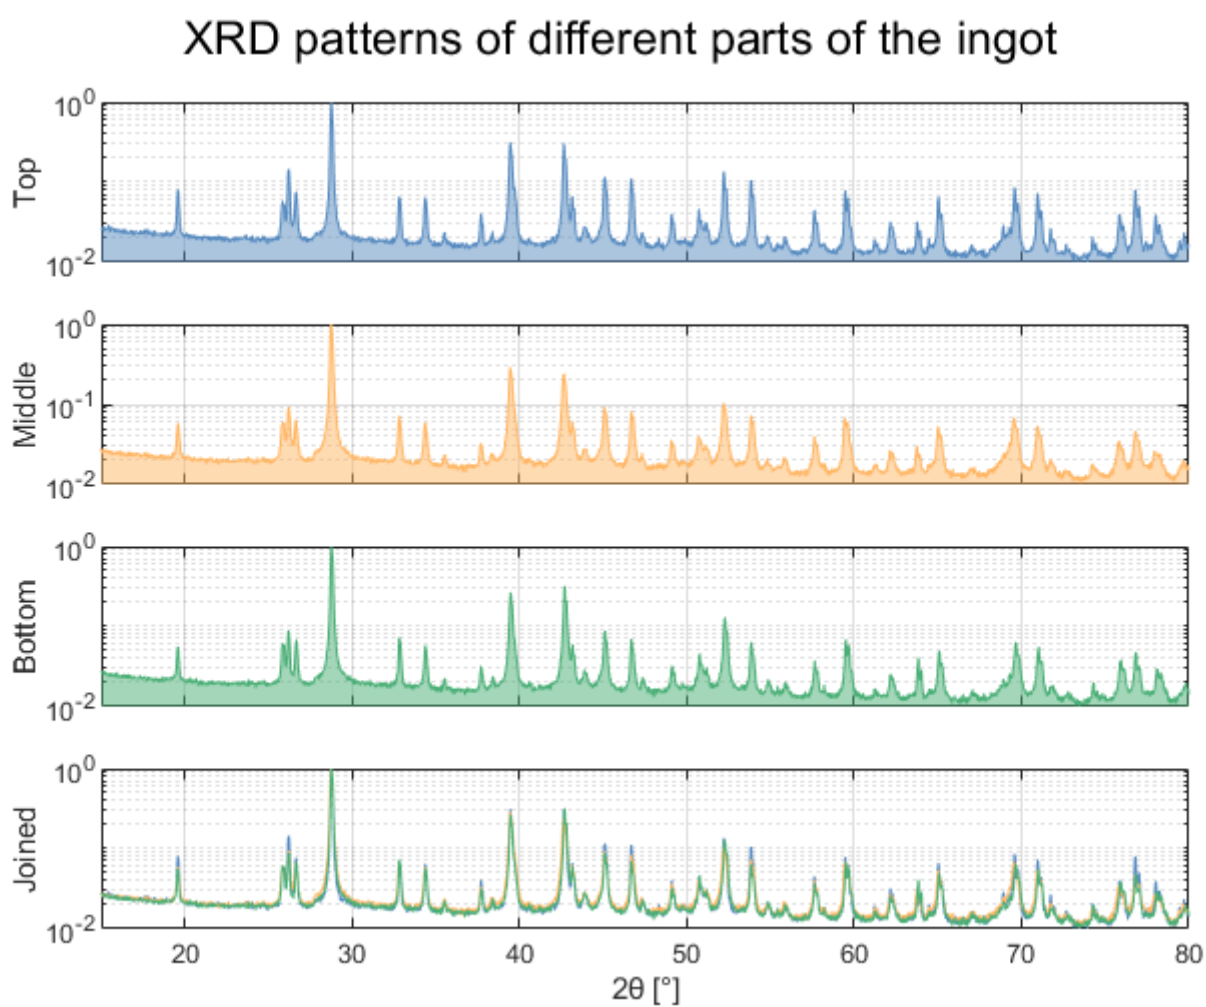

*Figure S1: Additional XRD spectra of the synthesized ingot. The uniformity of the target is confirmed by the overlapping graphs.*

## S2: Detailed structural analysis of STEM pictures

In this section, we present a more detailed analysis of the HAADF-STEM images of the MST single grain.

To begin, we study the in-plane intensity variations of each atomic plane. As can be seen from **Figure S2.1**, regardless of the atomic plane, the contrast remains fairly constant. This observation suggests that, while our sample exhibits an asymmetric distribution of antisites along the crystallographic c-axis (as explained in the main text), they are uniformly distributed in-plane. This differs from the observation of Y. Liu et al [Yaohua Liu et al. “Site mixing for engineering magnetic topological insulators”. In: Physical Review X 11.2 (2021), p. 021033.], which shows in-plane intensity variations in the Mn planes indicative not only of Mn-Sb site-mixing but also of their non-uniformity within each atomic plane.

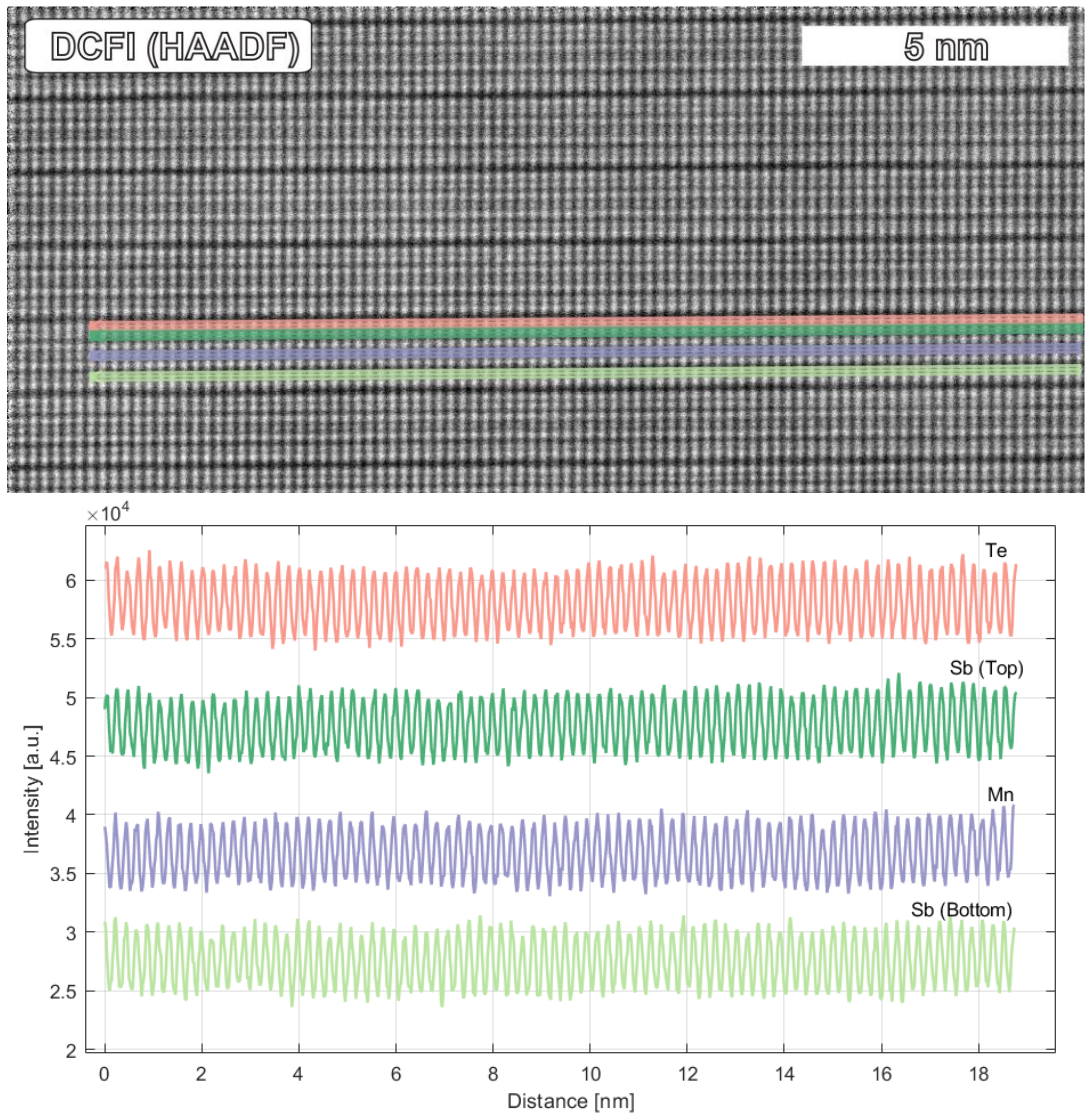

*Figure S2.1: In-plane intensity variation of a single MST grain. All the atomic layers show a fairly uniform contrast indicative of a homogeneously in-plane sample. Only vertical offsets were applied to the intensities.*

Next, the STEM-HAADF images were analyzed using the Atomap Python library [<https://atomap.org/>]. In the analysis, 2-D Gaussian functions are fitted to every atomic column, which allows for the quantification of interplanar distance perpendicular to the vdW gap; the results are illustrated in **Figure S2.2**.

Unlike the compositional asymmetry reported in section 3.1 of the main text, no structural asymmetry could be systematically determined between the different planes composing a single septuplet layer. Thus, it appears that the difference in site mixing between the Sb planes is small enough to not introduce significant strain.

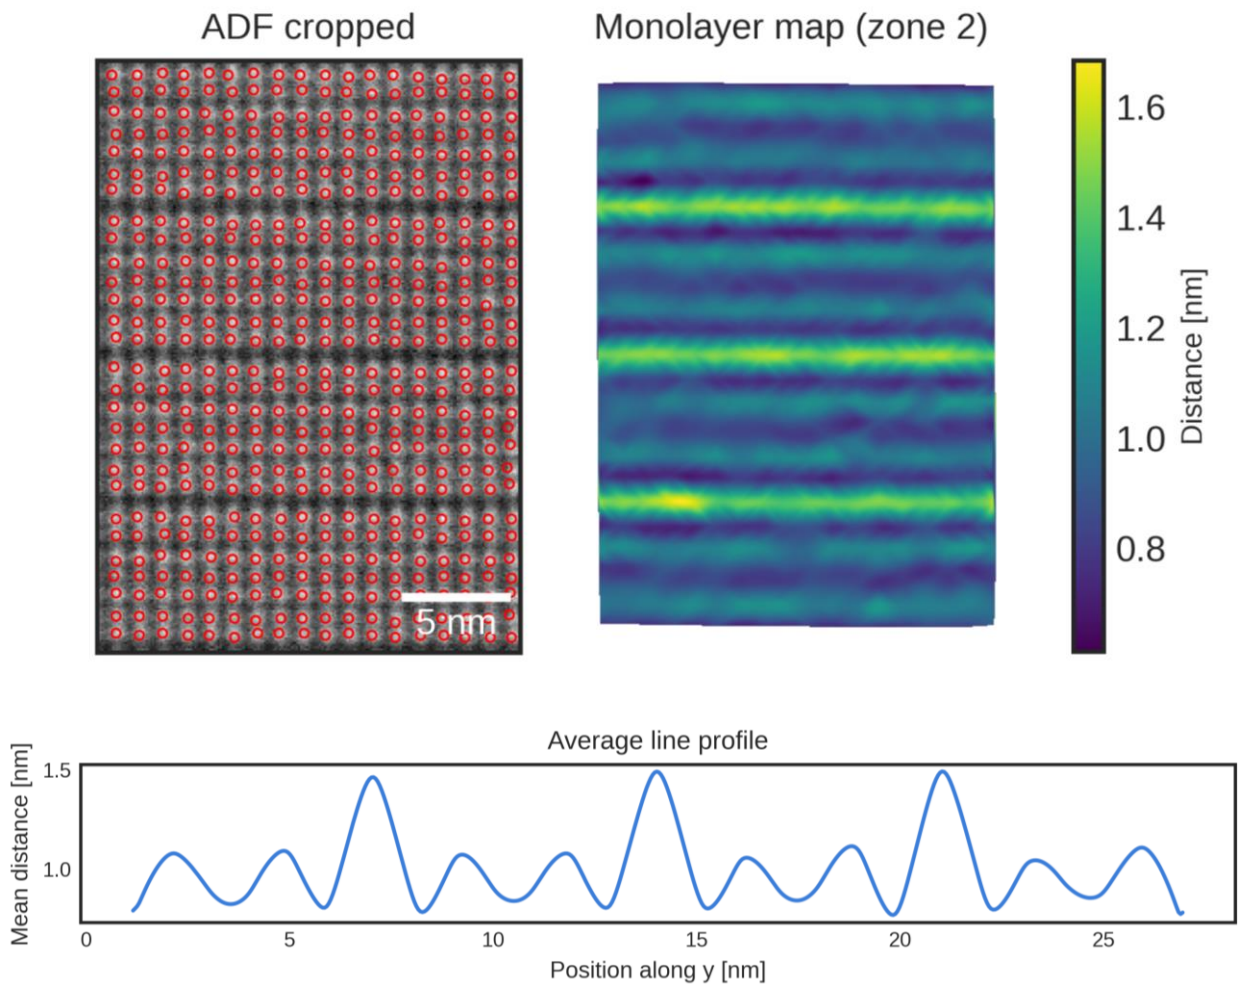

*Figure S2.2: Analysis of STEM-HAADF images using the Atomap Python library. The atomic positions are found by fitting 2-D gaussians. The large separation in interplanar distance corresponds to the vdW-like gap. No systematic structural asymmetry could be determined within a single septuplet layer.*

### S3: RHEED data of additional thin film depositions

In this section, we present the results of in-situ RHEED measurements during film growth.

#### S3.1: Seeding layer of MST.

Our attempts to use MST as the seeds are shown in **Figures S3.1.1 and S3.1.2**. The experiments consisted of depositing MST at room temperature (30°C) in an Ar atmosphere with a process pressure of 1.2E-1mbar, using 1J/cm<sup>2</sup> fluence. The RHEED pattern displayed at Time: 0.00s (see **Figure S3.1.1**) shows no particular features as expected from an amorphous SiO<sub>x</sub> substrate. As the film grows, the pattern starts to display ring-like features indicative of the presence of nanocrystals in the substrate. The situation is similar to Sb<sub>2</sub>Te<sub>3</sub> seeds (as will be shown in **Section S3.2**) and Bi<sub>2</sub>Te<sub>3</sub> [Vermeulen. “Growth and nanostructure of tellurides for optoelectronic, thermoelectric and phase-change applications”. English. PhD thesis. University of Groningen, 2019. isbn: 978-94-034-1422-5. Daniel Yimam. “Phase-change thin films growth and functionality: towards phase-change memory and reconfigurable nanophotonics”. English. PhD thesis. University of Groningen, 2023. doi: 10.33612/diss.622460932].

The final thickness of the film was determined to be around 4nm, which corresponds to a growth rate of 1nm for 100 pulses. This rate was determined by previous experiments using an Atomic Force Microscope [AFM], where the film was gently scratched with plastic tweezers and the thickness of the scratch was measured.

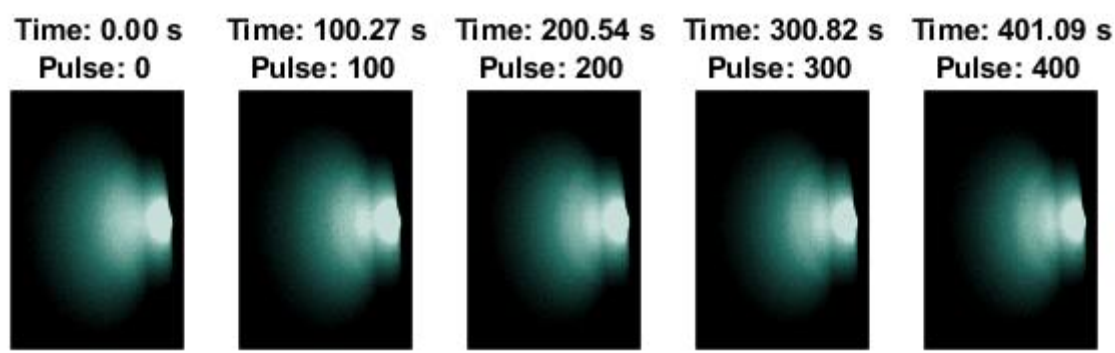

*Figure S3.1.1: RHEED data of an MST film grown at room temperature over an amorphous SiO<sub>x</sub>. The patterns show ring-like features indicative of nanocrystals.*

Once the deposition finished, the film was heated up to 210°C. As can be seen from **Figures S3.1.2**, the ring-like features begin to disappear past 120°C, and by 210°C the pattern once again shows no diffraction, similar to the amorphous SiO<sub>x</sub>. Even if the film is heated to 300°C, the pattern remains unchanged.

Therefore, it is likely that thin layers of MST evaporate before crystallizing, thereby hindering the formation of seeds and thus homoepitaxy.

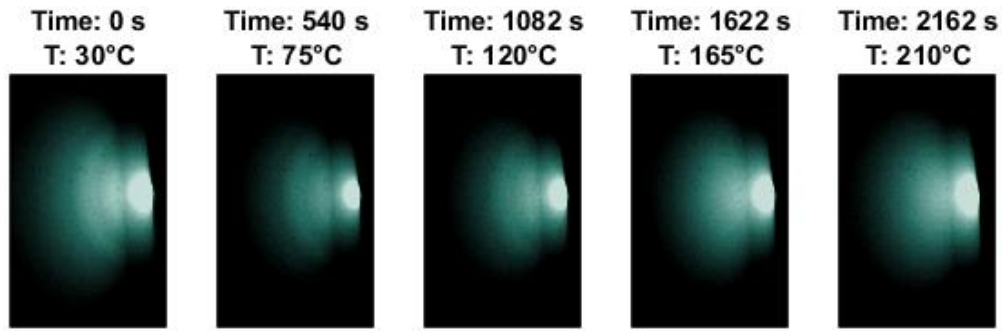

*Figure S3.1.2: Attempt at crystallization of an MST film (400 pulses). No crystallization occurs even when the sample was heated passed 300°C degrees as indicated by the absence of any diffraction.*

### S3.2: Van der Waals epitaxy and thickness limitation.

Next, we show the in-situ RHEED for the heteroepitaxy of MST over  $\text{Sb}_2\text{Te}_3$  seeds. **Figure S3.2.1** shows the room temperature of  $\text{Sb}_2\text{Te}_3$  over amorphous  $\text{SiO}_x$ . Similar to MST, the pattern also develops rings indicative of nanocrystals, just like **Figure S3.1.1**.

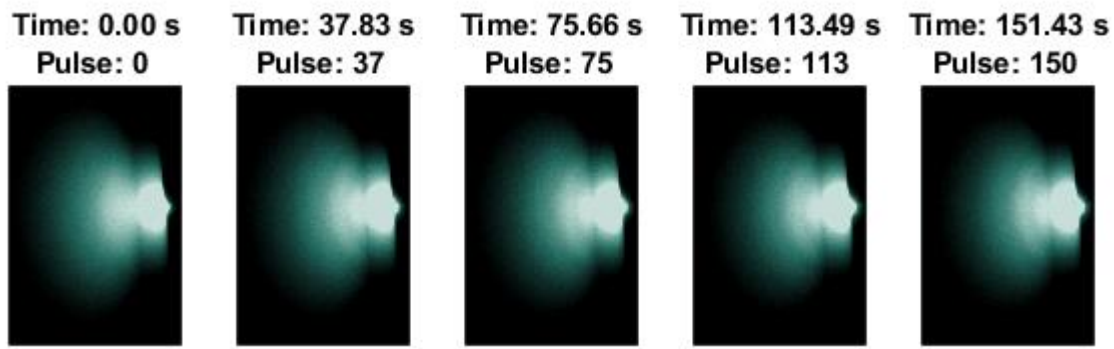

*Figure S3.2.1: RHEED data of an  $\text{Sb}_2\text{Te}_3$  film grown at room temperature over an amorphous  $\text{SiO}_x$ . The patterns show ring-like features indicative of nanocrystals.*

**Figure S3.2.2** shows the crystallization process of those seeds upon annealing. Around 170°C, the RHEED pattern develops streaks indicating that the  $\text{Sb}_2\text{Te}_3$  has crystallized with an out-of-plane texture. As the temperature increased, the features became more defined. The streak intensity is modulated, suggesting a multi-level surface [Ichimiya, A., & Cohen, P. I. (2004). Reflection high-energy electron diffraction. Cambridge University Press].

Before continuing the growth, a waiting period of 10 minutes was employed to stabilized the temperature feedback-loop. **Figure S3.2.3** shows the RHEED pattern for the first 600 pulses. The pattern remains qualitatively similar, but loses intensity over time, as expected from increased roughness and disorder.

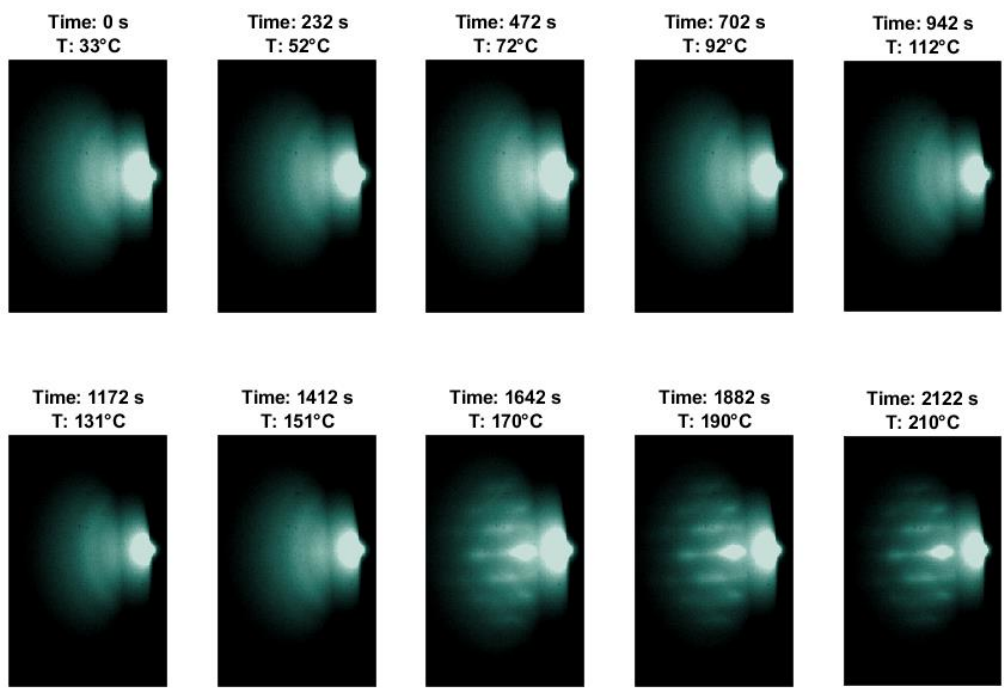

*Figure S3.2.2: RHEED pattern showing the crystallization of  $\text{Sb}_2\text{Te}_3$  seeds after annealing. The appearance of streaks indicates that the film is highly textured.*

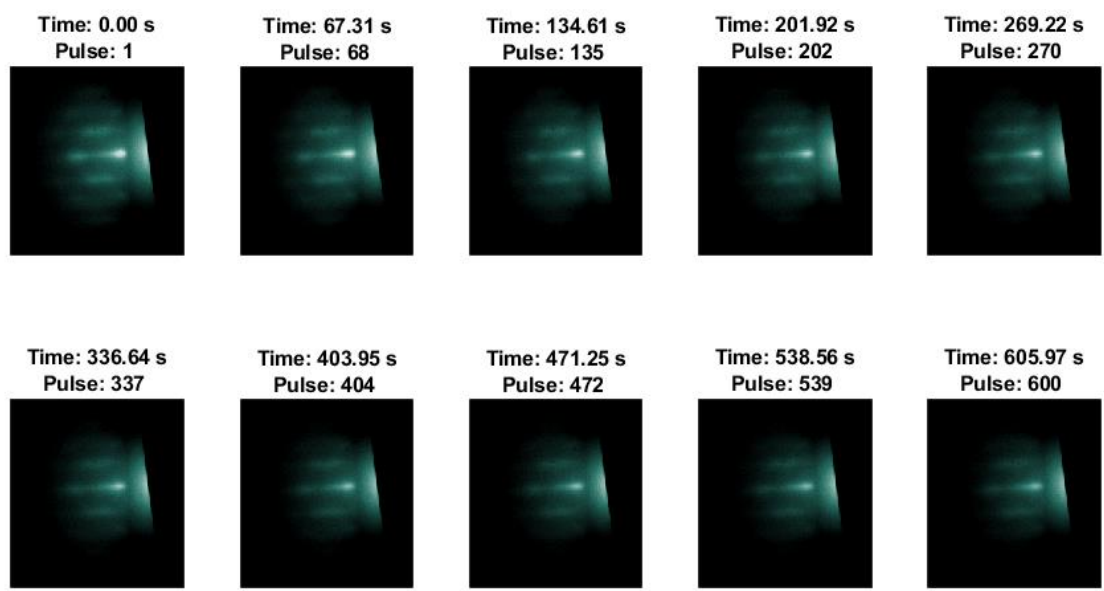

*Figure S3.2.3: RHEED pattern during the growth of MST over  $\text{Sb}_2\text{Te}_3$ . At the beginning of the growth, the RHEED streaks are preserved, indicating epitaxy. The intensity of the pattern diminishes as roughness and disorder increase.*

To qualitatively analyze the pattern, the pixel intensities are summed parallel to the direction of the RHEED streak and studied as a function of time. The process is illustrated in **Figure S3.2.4**. The position of the steaks is determined by subtracting a 4<sup>th</sup>-order polynomial background and fitting parabolas to the apex of the peaks, as illustrated in **Figure S3.2.5** for the pure  $\text{Sb}_2\text{Te}_3$  seeds and the 600<sup>th</sup> pulse of MST.

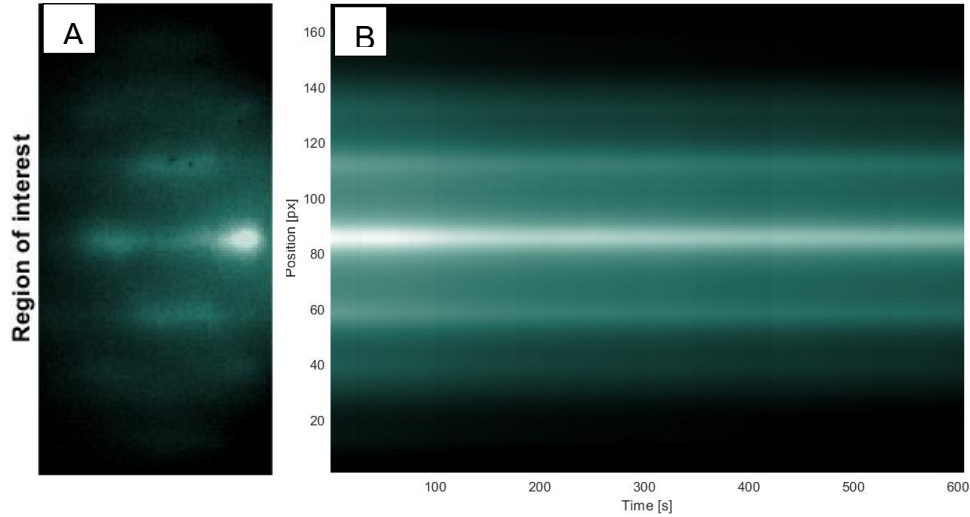

Figure S3.2.4: (A) Region of Interest in the diffraction pattern used to study the development of strain and RHEED oscillations. (B) Integrated intensities along the streaks and their intensity variations over time.

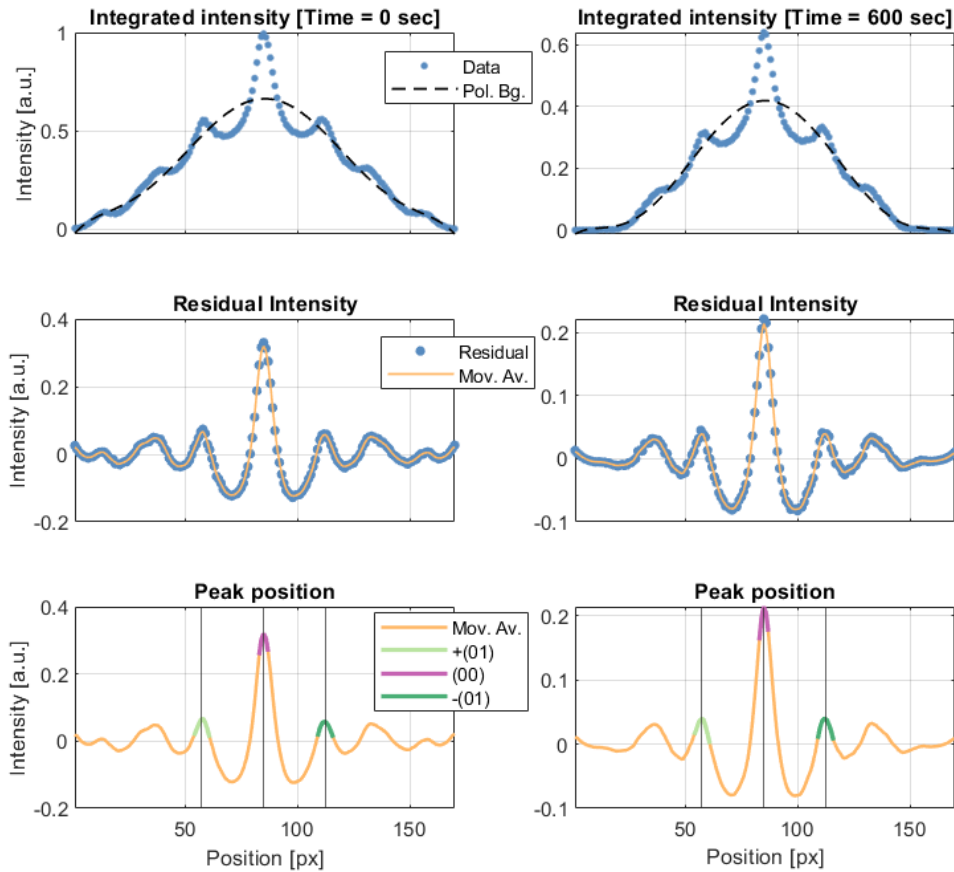

Figure S3.2.5: To study the stress developed during the growth, the position of the streaks is monitored as a function of time. The peaks are found by a quadratic fitting of the maximum after a polynomial background subtraction.

The average separation between the (01) [both left and right] and (00) streaks is plotted in **Figure S3.2.6 (B)**. The distance has a minimal increase (less than  $\frac{1}{2}$  a pixel) as the film grows consistent with the lattice-matched condition of the  $\text{Sb}_2\text{Te}_3$  seeds. The

slight increase points to a shrinkage of the crystal structure consistent with the relaxation of strain built during seeding [Vermeulen. “Growth and nanostructure of tellurides for optoelectronic, thermoelectric and phase-change applications”. English. PhD thesis. University of Groningen, 2019. isbn: 978-94-034-1422-5].

The intensity variation of the (00) streak, as determined by averaging the 5 pixels next to the apex, is plotted in **Figure S3.2.6 (A)**. Due to the many grains created during seeding, layer-by-layer growth is not expected; nevertheless, slight intensity oscillations can still be observed, further confirming the results of Van der Waals epitaxy. Note that because the growth is multilevel, the oscillation period does not necessarily indicate the completion of a full layer.

Finally, as the growth progressed, the pattern slowly changed to that presented in **Figure S3.2.7**. The appearance of rings superimposed on the RHEED streaks indicates the presence of particulate/nanocrystals carried by the plume as discussed in section 2.2 of the main text. This stopped epitaxy and thus limited the final film thickness obtained with this procedure.

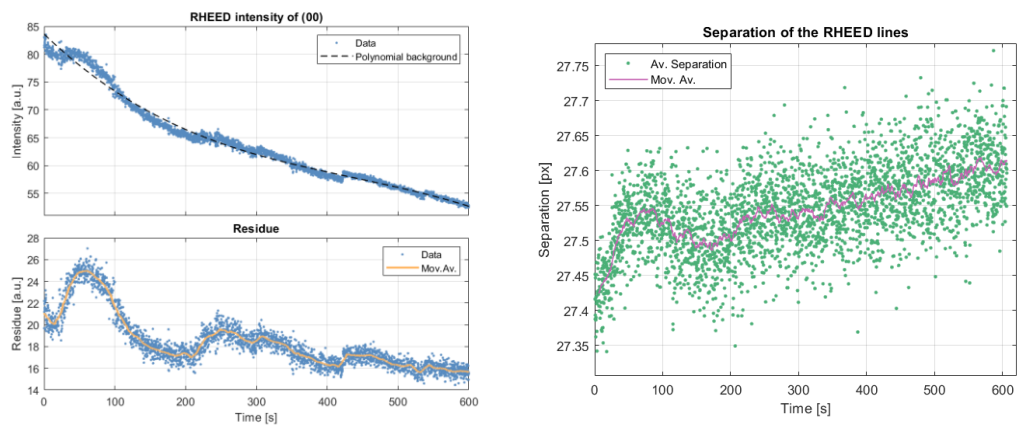

**Figure S3.2.6:** (A) Intensity variations of the (00) streak. Courtesy of the many Sb<sub>2</sub>Te<sub>3</sub> seeds, the growth is not layer by layer but multilevel; nevertheless, small oscillations can be observed, corroborating epitaxy. (B) Average separation between the (00) streak and (01) streak and its moving average. The separation increases very slightly (less than ½ a pixel change), consistent with less strain layers at the surface.

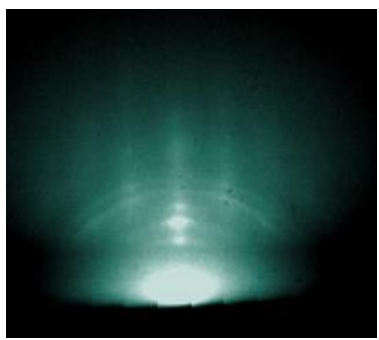

**Figure S3.2.7:** Around the 1000<sup>th</sup> pulse, the RHEED pattern slowly changes to a mixture of two diffraction patterns: streaks and rings. This superposition indicates the presence of nanocrystals on top of a textured film.

#### S4: EDS of solid ingot

To further study the stoichiometry and uniformity of the ingot at a micron-scale, the EDS spectra was measured. **Figure S4.1** shows the identified phases using EDAX TEAM: Texture & Elemental Analytical Microscopy software. The individual signal of the elements composing  $\text{MnSb}_2\text{Te}_4$  is illustrated in **Figure S4.2**; the minimal contrast indicates that those elements are in similar proportions all through the specimen, further corroborating the phase uniformity.

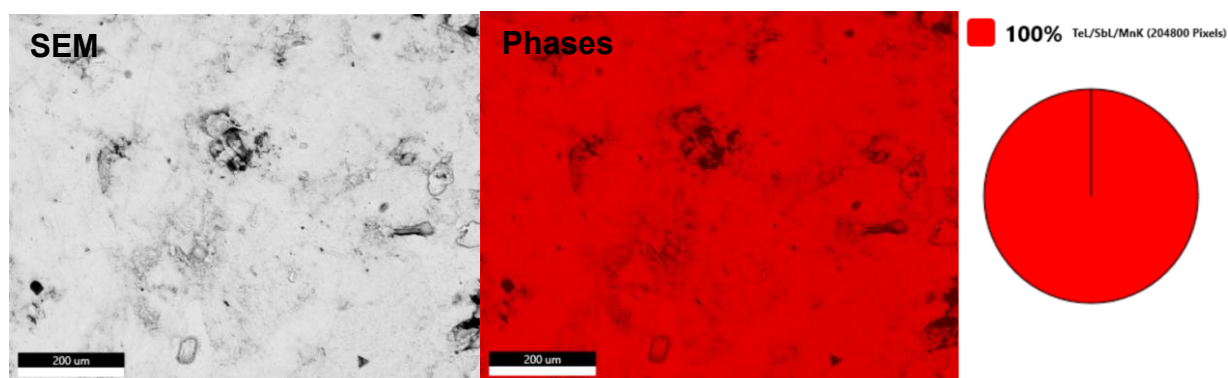

*Figure S4.1: Micrograph of the ingot's polished surface and phase map its corresponding phase map. No additional phases were identified.*

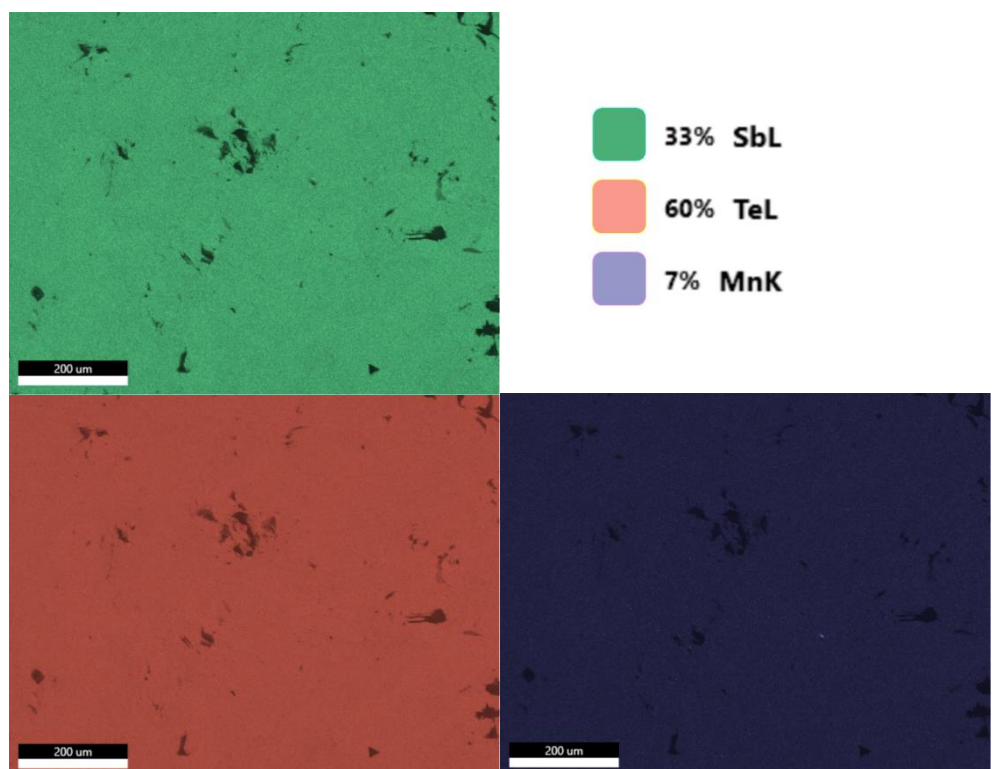

*Figure S4.2: Elemental Overlay of the EDS signal for Sb L-line, Te L-line, and Mn K-line with their respective weight percentage. The uniform intensity of the images indicates that the elements are equally distributed through the material.*

To estimate the composition of the ingot, the EDS spectrum was deconvoluted using the ZAF procedure [Newbury, D. E., & Ritchie, N. W. (2015). Performing elemental microanalysis with high accuracy and high precision by scanning electron microscopy/silicon drift detector energy-dispersive X-ray spectrometry (SEM/SDD-EDS). Journal of materials science, 50(2), 493-518.] as implemented in the EDAX TEAM software. The spectrum and its respective deconvolution are graphed in **Figure S4.3**. Additional elemental peaks of background origin were also included in the deconvolution.

The resulting atomic and weight percentages are summarized in **Table S4**; the stoichiometry is in good agreement with the expected composition of  $\text{MnSb}_2\text{Te}_4$  (Atomic: 14.28% Mn, 28.57% Sb, 57.14%).

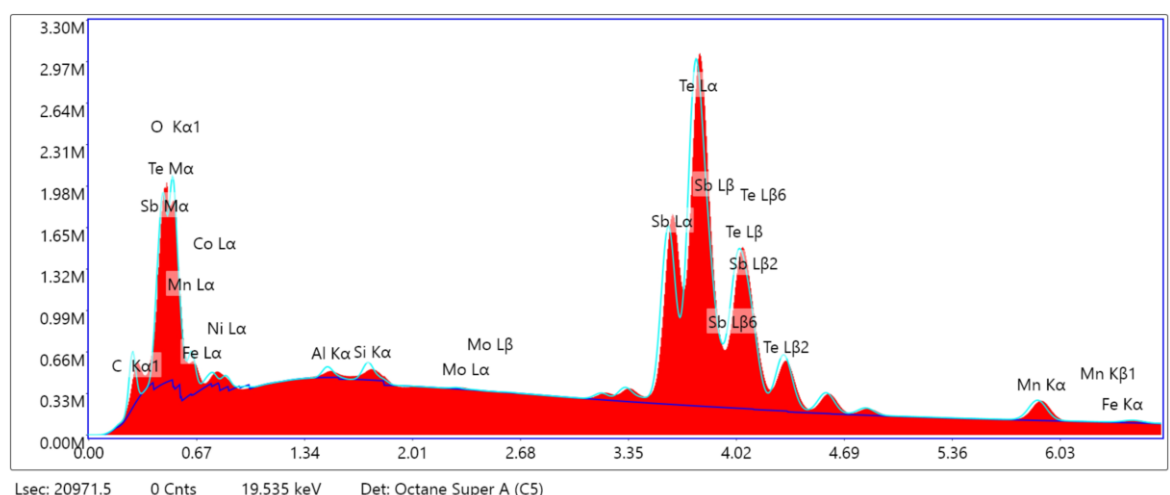

*Figure S4.3: Deconvolution of the total SEM-EDS spectra. Additional background elements (C, O, Fe, Ni, Al, Mo) were included in the deconvolution but excluded form quantification.*

| eZAF Smart Quant Results |         |         |          |         |        |        |        |        |
|--------------------------|---------|---------|----------|---------|--------|--------|--------|--------|
| Element                  | Weight% | Atomic% | Net Int. | Error % | Kratio | Z      | A      | F      |
| SbL                      | 29.60   | 28.03   | 1490.50  | 2.98    | 0.2868 | 1.0033 | 1.0003 | 1.0046 |
| TeL                      | 63.38   | 57.26   | 2728.40  | 3.07    | 0.5929 | 0.9720 | 1.0010 | 1.0006 |
| MnK                      | 7.01    | 14.71   | 211.90   | 5.86    | 0.0831 | 1.2978 | 0.9398 | 1.0109 |

*Table S4: Results of performing a ZAF analysis on the spectrum in Figure S5.3.*

## S5: Additional atomically-resolved EDS maps

### S5.1: Ingot

In this section, we present additional EDS maps of a single grain of MST. The results are represented in **Figure S5.1**. The measurements were done on a region different from **Figure 3b** of the main text and further corroborate the presence of an asymmetry in the anti-site distribution of Mn in the Sb planes. The structure is observed in all septuple layers. Once again, no site mixing was observed in the Te planes.

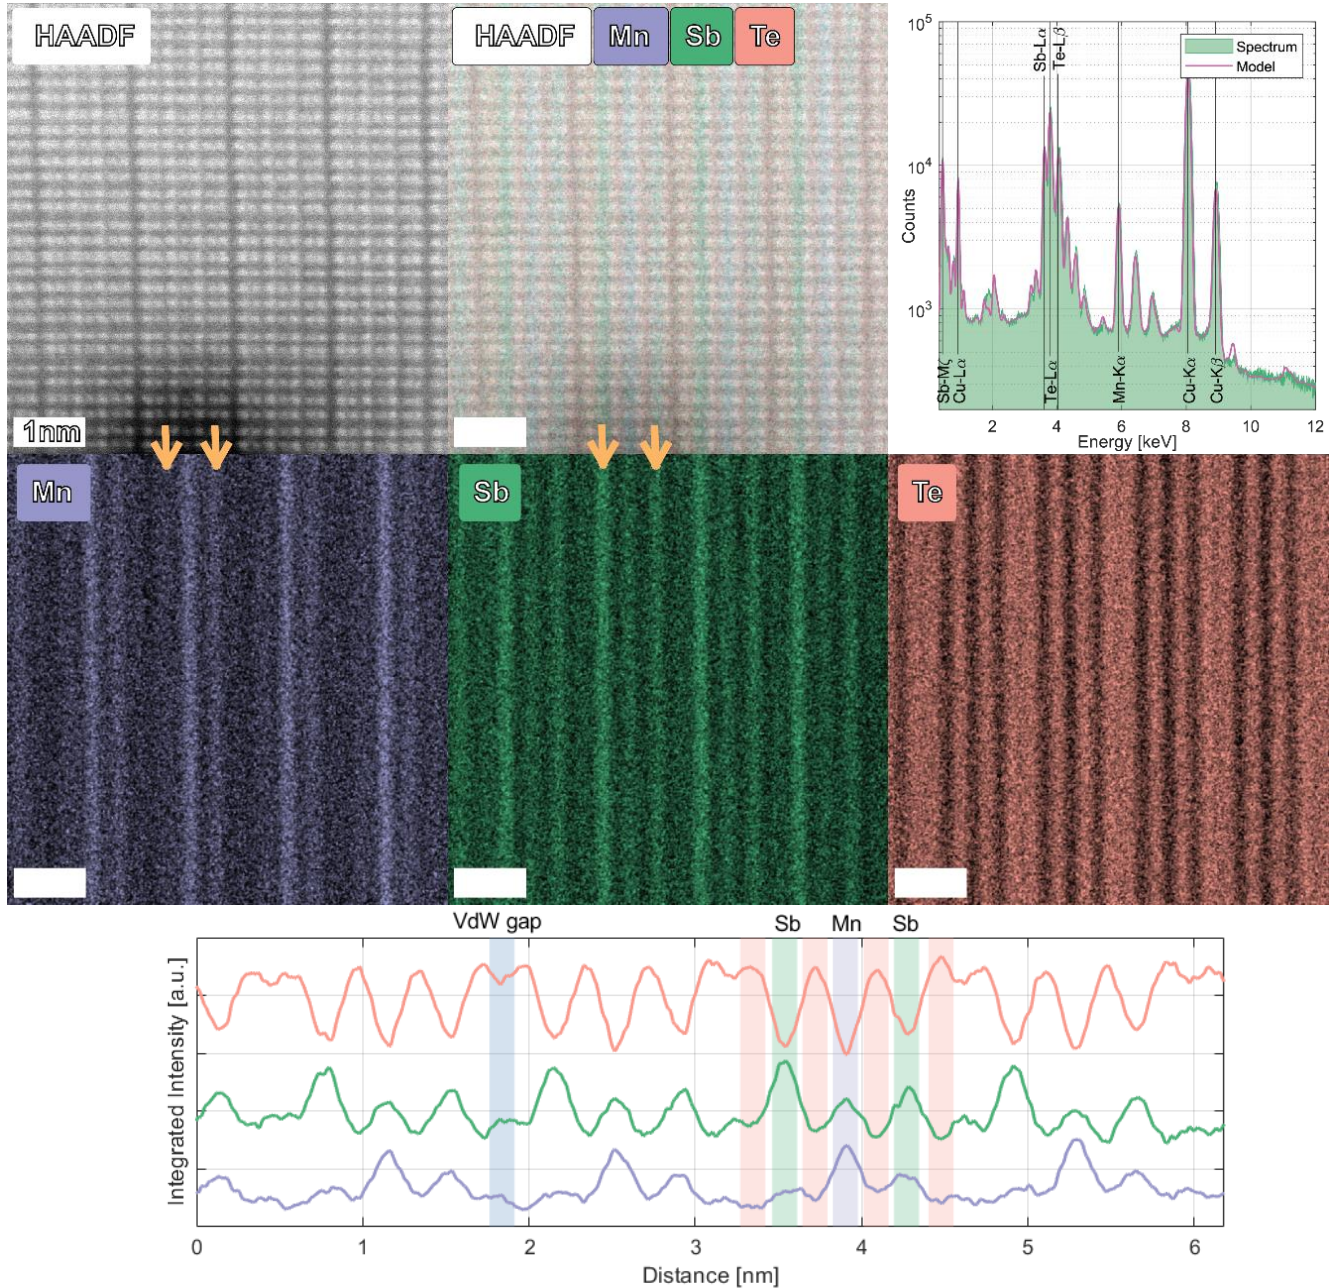

**Figure S5.1:** Additional atomically-resolved EDS-STEM scan (integration over 1092 frames). The measurements were taken over a different region than the one presented in Figure 3a of the main text. Mn-Sb site mixing is confirmed at the atomic scale. The asymmetry between the Sb-planes, marked with orange arrows, is clearly visible.

## S5.2: Additional information on Figure 3

In this section, we present additional analysis on the results presented in **Figure 3** of the main text regarding the single-grain stoichiometry. The total spectrum and its deconvolution are illustrated in **Figure S5.2.1**. The composition was estimated using the Brown–Powell ionization cross-section model as implemented in the Velox Software after a multi-parabolic background correction.

The resulting atomic and weight percentages are summarized in **Table S5.2.1**; the deconvolution is complicated by the fact that Sb-L and Te-L peaks present a significant overlap, thereby considerably increasing the uncertainties in the quantification of those particular elements. Overall, the stoichiometry (atomic: 17.5% Mn, 27.1% Sb, 55.4%) is in good agreement with the results presented in Figure 3d, if slightly Mn-rich.

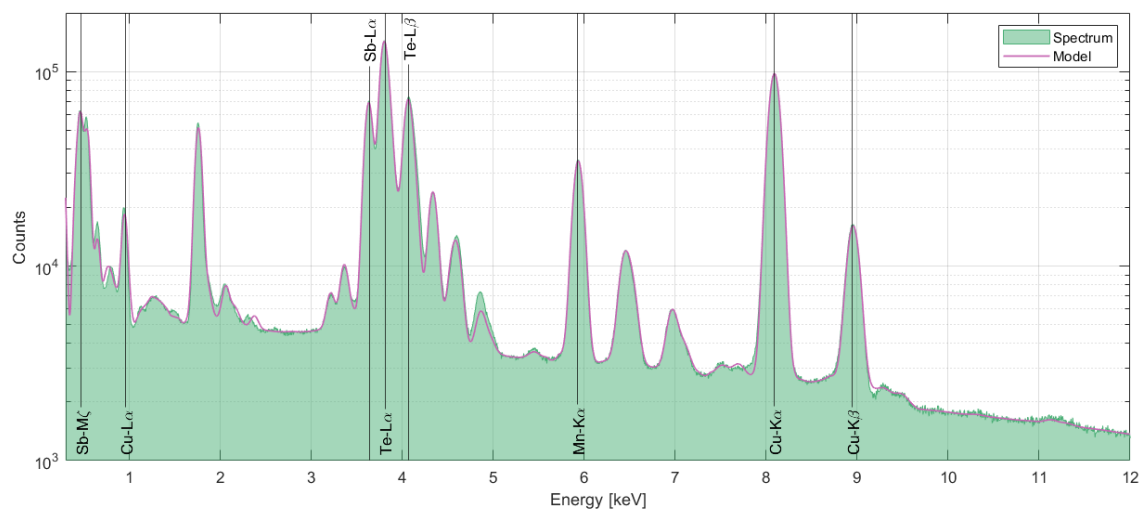

*Figure S5.2.1: Deconvolution of the total spectrum of Figure 3a of the main text. Additional background elements (C, O, Si, Ti, Cr, Fe, Co, Ni, Cu, Ga, Zr, Pt) were included in the deconvolution but excluded from quantification.*

| Velox analysis of spectrum (Brown – Powell model) |         |        |                     |                  |                   |                |               |
|---------------------------------------------------|---------|--------|---------------------|------------------|-------------------|----------------|---------------|
| Z                                                 | Element | Family | Atomic Fraction (%) | Atomic Error (%) | Mass Fraction (%) | Mass Error (%) | Fit error (%) |
| 25                                                | Mn      | K      | 17.50               | 1.29             | 8.49              | 0.70           | 0.2           |
| 51                                                | Sb      | L      | 27.13               | 2.73             | 29.16             | 3.03           | 0.05          |
| 52                                                | Te      | L      | 55.37               | 3.21             | 62.35             | 3.28           | 0.01          |

*Table S5.2.1: EDS Quantification of Figure S5.2.1.*

To further quantify the asymmetry between the Sb planes, the spectra recorded from only those planes are studied, as illustrated in **Figure S5.2.2**. The asymmetry between Sb-Mn site mixing is clearly resolved in the Sb-L $\alpha$  and Mn-K $\alpha$  peaks. The quantification of those areas is summarized in **Table S5.2.2**. Note that due to a considerable contribution of the rest of the crystal as a background signal, the percentual differences

between those two areas do not represent a direct measurement of the Mn/Sb percentual occupancies in those planes.

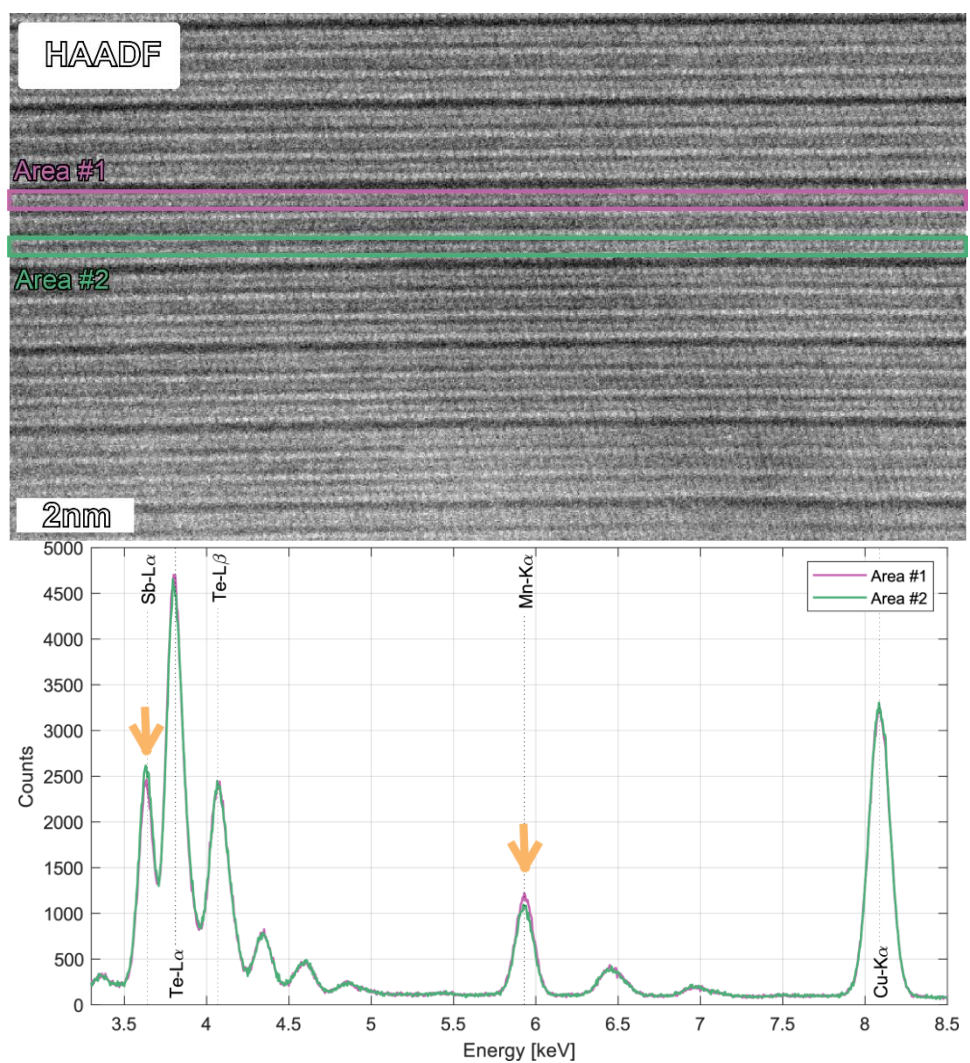

Figure S5.2.2: Comparison between the two Sb planes. By taking similar areas, the Cu-K $\alpha$  peak is normalized. The asymmetry in Sb and Mn concentration clearly resolved in the Sb-L $\alpha$  and Mn-K $\alpha$  peaks.

| Velox analysis of spectrum (Brown – Powell model) |         |        |                     |                  |                   |                |               |
|---------------------------------------------------|---------|--------|---------------------|------------------|-------------------|----------------|---------------|
| Z                                                 | Element | Family | Atomic Fraction (%) | Atomic Error (%) | Mass Fraction (%) | Mass Error (%) | Fit error (%) |
| <b>Area #1</b>                                    |         |        |                     |                  |                   |                |               |
| 25                                                | Mn      | K      | 17.83               | 1.29             | 8.67              | 0.70           | 0.07          |
| 51                                                | Sb      | L      | 28.32               | 2.79             | 30.52             | 3.10           | 0.02          |
| 52                                                | Te      | L      | 53.85               | 3.24             | 60.81             | 3.34           | 0.05          |
| <b>Area #2</b>                                    |         |        |                     |                  |                   |                |               |
| 25                                                | Mn      | K      | 16.08               | 1.18             | 7.74              | 0.63           | 0.16          |
| 51                                                | Sb      | L      | 30.89               | 2.96             | 32.96             | 3.25           | 0.08          |
| 52                                                | Te      | L      | 53.03               | 3.31             | 59.30             | 3.43           | 0.05          |

Table S5.2.2: EDS Quantification of the areas marked in Figure S5.2.2.

### S5.3: Thin film

In this section, we present the EDS-STEM results of the MST film over  $\text{Sb}_2\text{Te}_3$  seed; the results are summarized in **Figure 5.3**. Because the film was composed of small grains, elemental atomic resolution could not be obtained; nevertheless, the general distribution of the elements within a septuple layer could still be resolved. For instance, Mn appears to occupy only the middle layer of the septuple, while Sb populates both the Sb and Mn planes. The broadness of the Sb peaks also suggests some level of intermixing within the Te planes, but cannot be definitely concluded due to the poor signal-to-noise ratio.

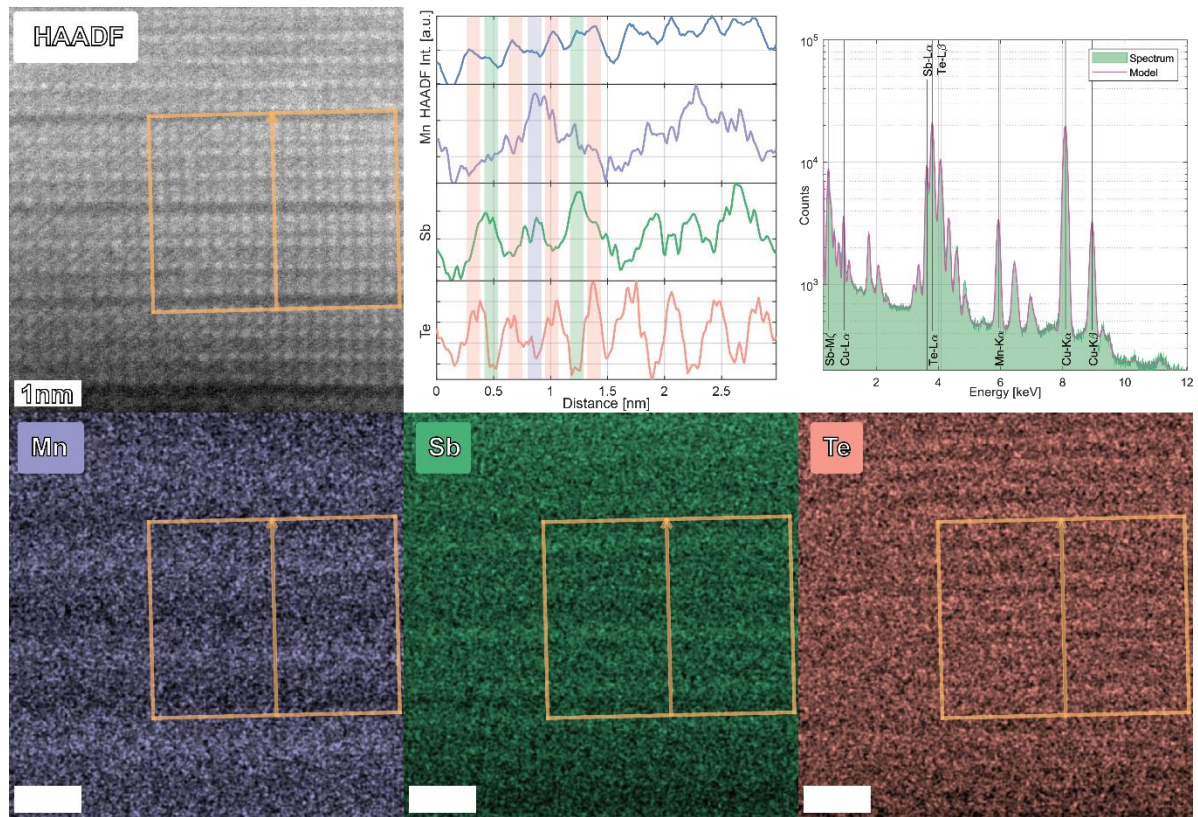

Figure S5.3: EDS-STEM elemental map of the MST film over  $\text{Sb}_2\text{Te}_3$  seeds. The Mn signal is mostly concentrated in the middle of the septuple, while Sb could be found both in the Sb and Mn planes.

## S6: Additional magnetization plots

In this section, we present the results of additional field cooling experiments at different fields. For weak field strengths, the magnetization develops a maximum as indicated in the main text (section 4). **Figure S6** shows that when the magnitude of the field increases, the maximum shifts to lower temperatures until it fully disappears at a moderate field strength. Indeed, at a value of 0.5T, the feature is fully absent and the curve is reminiscent of a ferromagnet.

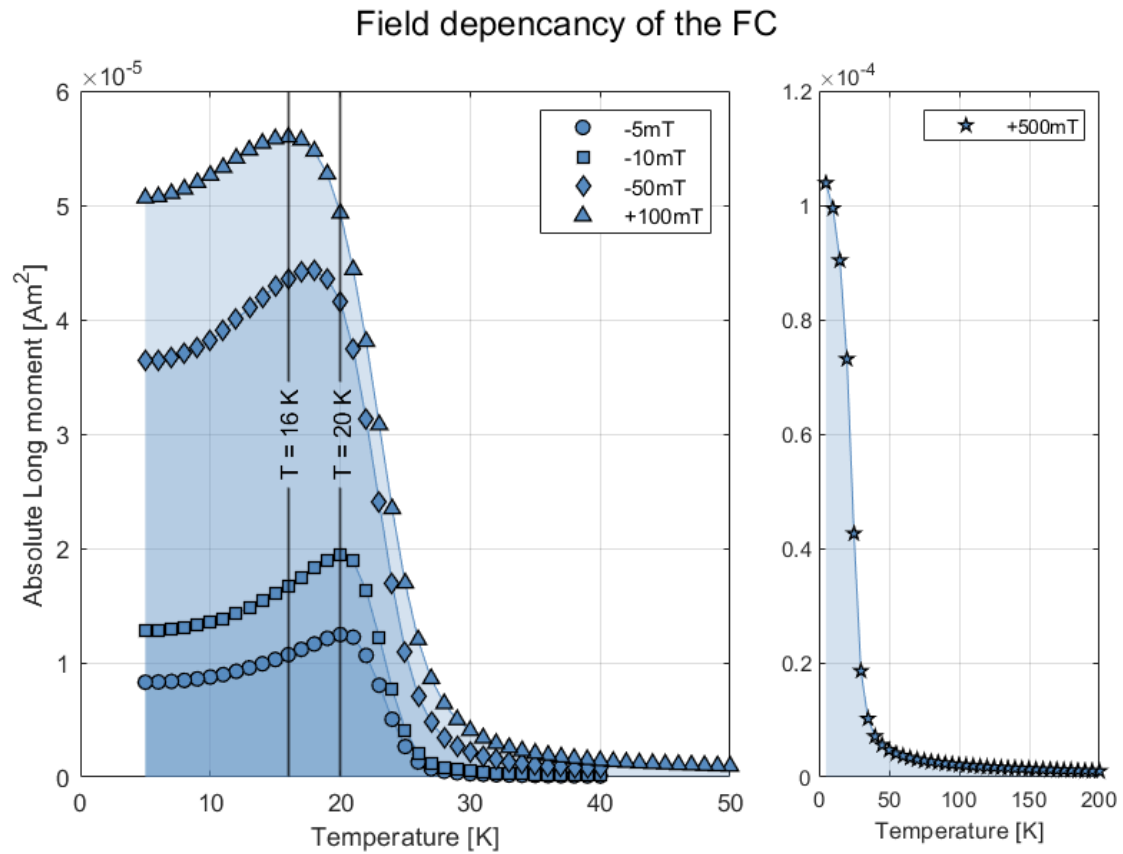

*Figure S6: Field dependency of the magnetization upon field cooling. The maximum shifts to lower values of temperature and eventually disappears at moderate field strength.*
